# Supplementary material for: Nanoscale lattice strains in self-ion implanted tungsten
Source: arXiv:2006.02657 ancillary file (2020-06-04)
Supplement: Supplementary file 1 [file SupplementaryInformation.pdf]

# Supplementary Information: Nanoscale lattice strains in self-ion implanted tungsten

N.W. Phillips[a*], H. Yu[a], S. Das[a], D. Yang[a], K. Mizohata[b], W. Liu[c], R. Xu[c], R.J. Harder[c], F. Hofmann[a+]

[a] *Department of Engineering Science, University of Oxford, Parks Road, Oxford, OX1 3PJ, UK*

[b] *Accelerator Laboratory, University of Helsinki, P.O. Box 64, 00560 Helsinki, Finland*

[c] *Advanced Photon Source, Argonne National Lab, 9700 S. Cass Avenue, Lemont, IL, USA*

[*] *Corresponding author E-mail address: nicholas.phillips@eng.ox.ac.uk (N.W. Phillips)*

[+] *Corresponding author E-mail address: felix.hofmann@eng.ox.ac.uk (F. Hofmann)*

## 1. Phasing of BCDI data

The following cycle was used for phasing BCDI data.

1. A guided phasing approach was applied [1, 2], consisting of 4 generations with an initial population of 40. Initially reduced resolution data was used. The initial phase guess was random. 'Best' results were selected using a sharpness metric [2], these were then averaged and used for the subsequent generation. 620 iterations were used in each generation, alternating between 20 iterations of ER and 180 iterations of HIO ($\beta = 0.9$) [3]. A shrinkwrap threshold [4] of 0.1 was applied to the object.
2. The result of cycle 1 was used to initialise this round of phasing. The parameters remained unchanged from cycle 1, except for the addition of a partial coherence correction [5] and all generations of data utilised the $146 \times 146 \times 212$ pixel array.
3. After up-sampling the result of cycle 2 to use as a start guess for the full $256 \times 256 \times 256$ pixel dataset, 20 iterations of ER followed by 180 iterations of HIO was repeated 15 times, followed by 1000 iterations of ER. The result was taken by averaging the final 50 iterations.
4. The previous cycle was then repeated using the result from cycle 3 as the start guess.

## 2. Supplementary Figures

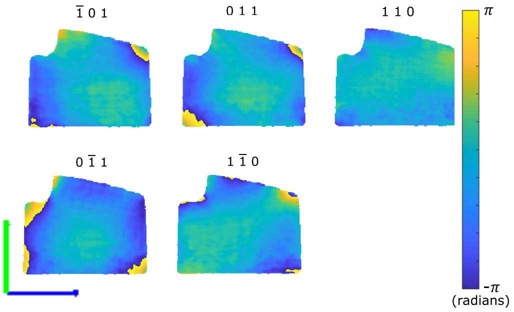


Supplementary Figure 1: Recovered phase through the vertical section (red - described in Figure 3 of the main text) for each of the five measured reflections. We note that the implantation layer is not clearly identifiable. The green and blue arrows are 500 nm long.

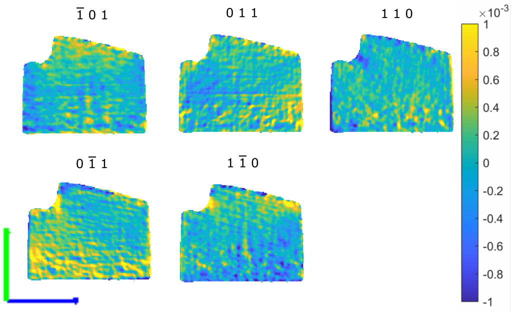


Supplementary Figure 2: Lattice strain on the vertical section (red - described in Figure 3 of the main text) shown in the direction of each scattering vector as recovered for each BCDI dataset. Note that the implantation layer is not as visible as it is when viewing the full strain tensor. The green and blue arrows are 500 nm long.

## 3. Supplementary Movies

Supplementary Movie 1: Lattice strain and rotation movie showing the slice-by-slice data recovered from MBCDI parallel to the vertical plane (red - described in Figure 3 of the main text). Shown are the six strain tensor components (upper right triangle and diagonal) alongside the three rotation tensor elements (bottom left triangle). The lattice swelling resulting from the implantation is most evident in the $\varepsilon_{yy}$ component. Heterogeneity of the strain within the implanted layer indicates damage induced evolution of the microstructure (particularly visible in the $\varepsilon_{xx}$, $\varepsilon_{yy}$ and $\varepsilon_{zz}$ components). The green and blue arrows are 500 nm long.

Supplementary Movie 2: Lattice strain and rotation movie showing the slice-by-slice data recovered from MBCDI parallel to the horizontal planes (green and black - described in Figure 3 of the main text). Shown are the six strain tensor components (upper right triangle and diagonal) alongside the three rotation tensor elements (bottom left triangle). The lattice swelling resulting from the implantation is most evident in the $\varepsilon_{yy}$ component. Heterogeneity of the strain within the implanted layer indicates damage induced evolution of the microstructure (particularly visible in the $\varepsilon_{xx}$, $\varepsilon_{yy}$ and $\varepsilon_{zz}$ components). The red and blue arrows are 500 nm long

Supplementary Movie 3: Isosurface movie of the recovered MBCDI strain microscopy sample with a strain isosurface plotted for the $\varepsilon_{yy}$ component using a value of $1 \times 10^{-3}$. The position of the previously viewed horizontal sections are shown by the green and black indicators.

## References

[1] C. C. Chen, J. Miao, C. W. Wang, T. K. Lee, Application of optimization technique to noncrystalline x-ray diffraction microscopy: Guided hybrid input-output method, Physical Review B - Condensed Matter and Materials Physics 76 (2007) 1–5.

[2] J. N. Clark, J. Ihli, A. S. Schenk, Y. Y. Kim, A. N. Kulak, J. M. Campbell, G. Nisbet, F. C. Meldrum, I. K. Robinson, Three-dimensional imaging of dislocation propagation during crystal growth and dissolution, Nature Materials 14 (2015) 780–784.

[3] J. R. Fienup, Phase retrieval algorithms: a comparison, Applied Optics 21 (1982) 2758.

[4] S. Marchesini, H. N. Chapman, S. P. Hau-Riege, R. A. London, A. Szoke, H. He, M. R. Howells, H. Padmore, R. Rosen, J. C. H. Spence, U. Weierstall, Coherent X-ray diffractive imaging: applications and limitations, Optics Express 11 (2003) 2344.

[5] J. N. Clark, X. Huang, R. Harder, I. K. Robinson, High-resolution three-dimensional partially coherent diffraction imaging, Nature Communications 3 (2012) 993.
